# Supplementary material for: Differential Diffusion: Giving Each Pixel Its Strength
Source: arXiv:2306.00950 source file (2024-02-28)
Supplement: Supplementary file 1 [file supp-exp-info.tex]

\section{Supplementary Experiments Information}

\input{methods/diffusion_extension}
\input{algs/diff-img2img-skipping}
\input{figs/eval/skipping_trend}
\input{tabs/skipping_time}
\input{figs/eval/single_reconstruction}
\begin{figure}
  \centering
\includegraphics[width=0.15\textwidth,frame]{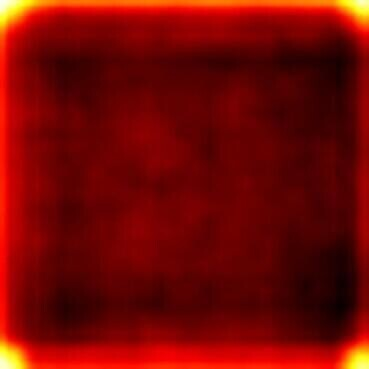}
\caption{This figure shows the perceptual similarity map's spatial bias.}
\label{fig:spatial_bias}
\end{figure}

\newcommand{\mm}{0.16\textwidth}

\begin{figure*}
  \centering
  \begin{tabular}{cc}
    \multirow{2}{*}{Map 1} & \includegraphics[width=0.3\textwidth, frame, valign=c]{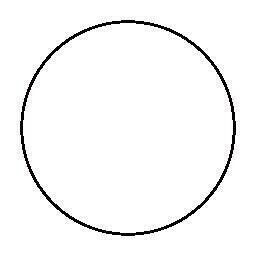} \\
    & \\
    \multirow{2}{*}{Map 2 / Metric} & 
    \begin{tabular}{ccc}
      \toprule
       & {CAM ($\uparrow$)} & {DAM ($\downarrow$)} \\
      \midrule
            \includegraphics[width=\mm, frame]{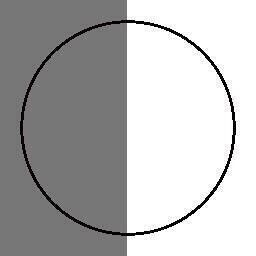} & \textbf{0.43} & 39.37\\ 
            \includegraphics[width=\mm, frame]{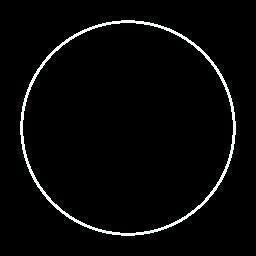} & -1 & \textbf{0} \\
                        \includegraphics[width=\mm, frame]{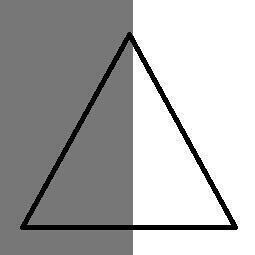} & 0.01 & 43.58 \\

      \bottomrule
    \end{tabular}
  \end{tabular}
  \caption{Comparison of CAM and DAM scores of map 1 to three map 2 options.
  }
\label{cam-dam-couterexample}
\end{figure*}

\input{figs/eval/user_study_screenshot}
